# Supplementary material for: ReynoldsFlow: Physics-Inspired Spatiotemporal Flow Representation for Video Understanding
Source: arXiv:2503.04500 source file (2026-08-20)
Supplement: Supplementary file 1 [file X_suppl.tex]

% \clearpage
% \setcounter{page}{1}
\maketitlesupplementary

\section{Methodology}
\label{sec:appendix_methodology}

\subsection{Helmholtz Decomposition}
Let \(\bm{v} \in C^1(V, \mathbb{R}^2)\) denote a continuously differentiable vector field. According to the Helmholtz decomposition theorem, \(\bm{v}\) can be uniquely expressed as the sum of an irrotational (curl-free) component and a solenoidal (divergence-free) component:  
\[
\bm{v} = \bm{v}_r + \bm{v}_o,
\]
where \(\bm{v}_r\) is curl-free, satisfying \( \nabla \times \bm{v}_r = 0 \), and \(\bm{v}_o\) is divergence-free, satisfying \( \nabla \cdot \bm{v}_o = 0 \). For conservative vector fields, these components can be described in terms of a scalar potential \(\phi\) and a vector potential \(\bm{A}\):  
\[
\bm{v}_r = \nabla \phi, \quad \bm{v}_o = \nabla \times \bm{A}.
\]  
This decomposition provides a principled framework for analyzing flow fields, making it particularly valuable for optical flow modeling and motion estimation tasks.

\subsection{Area transformation via Euler update}
Consider a position \(\bm{p} \in \mathbb{R}^2\) evolving over time \(t\) under the influence of a vector field \(\bm{v}\). Let \(t^n\) denote the discrete time at the \(n\)-th step, with a uniform time increment \(\Delta t = t^{n+1} - t^n\). The position at time \(t^n\) is \(\bm{p}^n = \begin{pmatrix} x^n \\ y^n \end{pmatrix}\), and the vector field evaluated at \(\bm{p}^n\) and \(t^n\) is \(\bm{v}^n = \begin{pmatrix} v_x^n \\ v_y^n \end{pmatrix}\). Using the explicit Euler method, the position update is:  
\[
\bm{p}^{n+1} = \bm{p}^n + \bm{v}^n(\bm{p}^n) \Delta t.
\]  
Or equivalently:  
\[
\begin{pmatrix}
x^{n+1} \\ y^{n+1}
\end{pmatrix} = 
\begin{pmatrix}
x^n \\ y^n
\end{pmatrix} + 
\begin{pmatrix}
v_x^n \\ v_y^n
\end{pmatrix} \Delta t.
\]  
Now consider the differential wedge product \(dx \wedge dy\) at \(\bm{p}^{n+1}\). Expanding this via the Euler update yields:  
\[
dx^{n+1} \wedge dy^{n+1} = \left(dx^n + dv_x^n dt\right) \wedge \left(dy^n + dv_y^n dt\right).
\]  
Simplifying:  
\begin{equation*}
    \begin{aligned}
        dx^{n+1} \wedge dy^{n+1} &= dx^n \wedge dy^n + dx^n \wedge dv_y^n dt \\
        &\hspace*{8mm} + dv_x^n dt \wedge dy^n + dv_x^n dt \wedge dv_y^n dt.
    \end{aligned}
\end{equation*}
Using the fact that \(dv_x = \frac{\partial v_x}{\partial x} dx + \frac{\partial v_x}{\partial y} dy\) and \(dv_y = \frac{\partial v_y}{\partial x} dx + \frac{\partial v_y}{\partial y} dy\), the expansion becomes:  
\[
dx^{n+1} \wedge dy^{n+1} = dx^n \wedge dy^n + \nabla \cdot \bm{v}^n \, dx^n \wedge dy^n \, dt + \mathcal{O}((dt)^2).
\]  
For sufficiently small \(\Delta t\), this simplifies to:  
\[
dx^{n+1} \wedge dy^{n+1} \approx \left(1 + \nabla \cdot \bm{v}^n \Delta t \right) dx^n \wedge dy^n.
\]

\subsection{Derivation of ReynoldsFlow}
Consider \(f = f(\bm{p}, t)\) as the grayscale intensity function in the Reynolds Transport Theorem, where \(\bm{p}\) denotes the spatial position in the image domain, and \(t\) corresponds to the time of the \(n\)-th frame. The theorem can be written as:
\begin{equation*}
    \begin{aligned}
        \frac{d}{dt}\int_{\Omega(t)} f \, dA &= \int_{\Omega(t)} \frac{\partial f}{\partial t} \, dA + \int_{\partial \Omega(t)} f (\bm{v} \cdot \bm{n}) \, dS \\
        \boxed{\text{Divergence Theorem}} &= \int_{\Omega(t)} \frac{\partial f}{\partial t} \, dA + \int_{\Omega(t)} \nabla \cdot (f \bm{v}) \, dA \\
        &= \int_{\Omega(t)} \left( \frac{\partial f}{\partial t} + \nabla f \cdot \bm{v} + f \nabla \cdot \bm{v} \right) \, dA.
    \end{aligned}
\end{equation*}

\subsubsection{Formulation of Optical flow}
Assume that \(\int_{\Omega(t)} f \, dV\) remains constant over time for all points \(\bm{p} \in \Omega(t)\), and that the vector field \(\bm{v}\) is divergence-free (\(\nabla \cdot \bm{v} = 0\)), we then have:
\[
0 = \int_{\Omega(t)} \left( \frac{\partial f}{\partial t} + \nabla f \cdot \bm{v} \right) \, dA.
\]  
For a patch image, this further simplifies to:  
\[
    \bm{v}^n_o = - (\nabla f)^{\dagger} \frac{\partial f}{\partial t},
\]  
which forms the basis for classical optical flow methods, such as the Lucas-Kanade or Horn-Schunck approach.

\subsubsection{Formulation of ReynoldsFlow}
Consider a broader perspective using the Reynolds Transport Theorem, where the vector field \(\bm{v}\) is not necessarily divergence-free. From the formulation:
\begin{equation*}
    \resizebox{\linewidth}{!}{$
    \begin{aligned}
        \frac{d}{dt}\int_{\Omega(t)}f \, dA &= \int_{\Omega(t)} \left( \frac{\partial f}{\partial t} + \nabla f \cdot \nabla \phi + \nabla f \cdot (\nabla \times \bm{A}) + f \Delta \phi \right) \, dA \\
    \end{aligned}
    $}
\end{equation*}
We can obtain:
\begin{equation*}
    \resizebox{\linewidth}{!}{$
    \begin{aligned}
        \text{LHS} &= \frac{1}{\Delta t} \left( \int_{\Omega^{n+1}}f^{n+1} \, dA^{n+1} - \int_{\Omega^n}f^n \, dA^n \right)\\
        \boxed{\text{Euler method}} &\approx \frac{1}{\Delta t} \int_{\Omega^n} \left[ (I + \nabla \cdot \bm{v}^n \Delta t) f^{n+1} - f^n \right] \, dA^n\\
        &= \int_{\Omega^n} \left(\frac{f^{n+1} - f^n}{\Delta t} + f^{n+1}\nabla \cdot \bm{v}^n \right) \, dA^n \\
        &\approx \int_{\Omega^n} \left(\frac{(f^n + \frac{\partial f^n}{\partial t}\Delta t + \nabla f^n \cdot \Delta \bm{p}^n) - f^n}{\Delta t} + f^{n+1}\nabla \cdot \bm{v}^n \right) \, dA^n \\
        \boxed{\Delta t\rightarrow 0}&\approx \int_{\Omega^n} \left(\frac{\partial f^n}{\partial t} + \nabla f^n \cdot \bm{v}^n + f^{n+1}\nabla \cdot \bm{v}^n \right)\, dA^n \\
        &= \int_{\Omega^n} \left(\frac{\partial f^n}{\partial t} + \nabla f^n \cdot (\bm{v}_r^n + \bm{v}_o^n) + f^{n+1}\nabla \cdot (\bm{v}_r^n + \bm{v}_o^n)\right)\, dA^n\\
        &= \int_{\Omega^n} \left(\frac{\partial f^n}{\partial t} + \nabla f^n \cdot \bm{v}_r^n + \nabla f^n \cdot \bm{v}_o^n + f^{n+1}\nabla \cdot \bm{v}_r^n \right)\, dA^n \\
        \boxed{\text{RHS}} &= \int_{\Omega^n} \left(\frac{\partial f^n}{\partial t} + \nabla f^n \cdot \bm{v}_r^n + \nabla f^n \cdot \bm{v}_o^n + f^{n}\nabla \cdot \bm{v}_r^n \right)\, dA^n. \\
    \end{aligned}
    $}
\end{equation*}
For a conservative field, there exists a potential \(\phi\) such that \(\bm{v}_r^n = \nabla \phi^n\), leading to the equation:
\[
\int_{\Omega^n} \delta f^n \Delta \phi^n \, dA^n = 0,
\]
where \(\delta f^n = f^{n+1} - f^n\). Additionally,
\begin{equation*}
    \resizebox{\linewidth}{!}{$
    \begin{aligned}
        \int_{\Omega^n} \delta f^n \Delta \phi^n \, dA^n &= \int_{\Omega^n} \delta f^n \nabla \cdot \nabla \phi^n \, dA^n \\
        &= \int_{\Omega^n}\left(\nabla \cdot \delta f^n\nabla \phi^n - \nabla \delta f^n \cdot \nabla \phi^n \right) \, dA^n \\
        &= \int_{\partial \Omega^n} \delta f^n \nabla \phi^n \cdot \bm{n} \, dS^n - \int_{\Omega^n} \nabla \delta f^n \cdot \nabla \phi^n  \, dA^n. \\
    \end{aligned}
    $}
\end{equation*}
This yields the following relation:
\[
\int_{\partial \Omega^n} \delta f^n \bm{v}_r^n \cdot \bm{n} \, dS^n = \int_{\Omega^n} \nabla \delta f^n \cdot \bm{v}_r^n \, dA^n.
\]

\subsection{Implementation Details}
To compute \(\bm{v}^r_n\) for a specific \(n\)-th frame, we start from the integral equation:  
\[
\int_{\partial \Omega^n} \delta f^n \bm{v}_r^n \cdot \bm{n} \, dS^n = \int_{\Omega^n} \nabla \delta f^n \cdot \bm{v}_r^n \, dA^n.
\]  
Here, \(f\) denotes a grayscale image of resolution \(w \times h\) pixels, with the upper-left corner defined as the origin. Assuming that \(\bm{v}^n_r\) is constant within a \(3 \times 3\) window, we approximate the boundary integral on the left-hand side (LHS) using Simpson's rule as:  
\begin{equation*}
    \begin{aligned}
        &\int_{\partial \Omega^n} \delta f^n \bm{v}_r^n \cdot \bm{n} \, dS^n = \left[(\delta f^n_{b})_x, (\delta f^n_{b})_y \right] \cdot \bm{v}_r^n \\
        &= \left[ \frac{1}{3} \begin{bmatrix}
            1 &  4 &  1\\
            0 &  0 &  0\\
           -1 & -4 & -1
       \end{bmatrix} * \delta f^n,
       \frac{1}{3} \begin{bmatrix}
        -1 &  0 &  1\\
        -4 &  0 &  4\\
        -1 &  0 &  1
    \end{bmatrix} * \delta f^n \right] \cdot \bm{v}_r^n,
    \end{aligned}
\end{equation*}  
where \((\delta f^n_{b})_x\) and \((\delta f^n_{b})_y\) are the boundary components in the \(x\)- and \(y\)-directions, respectively.
For the right-hand side (RHS), the domain integral can be expressed as:  
\begin{equation*}
    \begin{aligned}
        &\int_{\Omega^n} \nabla \delta f^n \cdot \bm{v}_r^n \, dA^n = [(\nabla \delta f^n)_x, (\nabla \delta f^n)_y] \cdot \bm{v}_r^n \\
        &= \left[\frac{1}{9} \begin{bmatrix}
            1 & 1 & 1\\
            1 & 1 & 1\\
            1 & 1 & 1
        \end{bmatrix} * \left(\frac{1}{2} \begin{bmatrix}
             0 & 0 & 0 \\
            -1 & 0 & 1 \\
             0 & 0 & 0
        \end{bmatrix} * \delta f^n \right), \right. \\
        &\hspace{8mm} \left. \frac{1}{9} \begin{bmatrix}
            1 & 1 & 1\\
            1 & 1 & 1\\
            1 & 1 & 1
        \end{bmatrix} * \left(\frac{1}{2} \begin{bmatrix}
             0 & -1 & 0 \\
             0 &  0 & 0 \\
             0 &  1 & 0
        \end{bmatrix} * \delta f^n \right) \right] \cdot \bm{v}_r^n.
    \end{aligned}
\end{equation*}  

By equating the LHS and RHS, we then obtain:  
\begin{equation*}
    \begin{aligned}
        &\int_{\Omega^n} \nabla \delta f^n \cdot \bm{v}_r^n \, dA^n - \int_{\partial \Omega^n} \delta f^n \bm{v}_r^n \cdot \bm{n} \, dS^n = 0 \\
        % &\Rightarrow [\nabla_x \delta f^n, \nabla_y \delta f^n] \cdot \bm{v}_r^n - \left[\delta f^n_{b x}, \delta f^n_{b y} \right] \cdot \bm{v}_r^n = 0 \\
        &\Rightarrow [(\nabla \delta f^n)_x - (\delta f^n_{b})_x, (\nabla \delta f^n)_y - (\delta f^n_{b})_y] \cdot \bm{v}_r^n = 0.
    \end{aligned}
\end{equation*}  
Finally, define \(\bm{v}^n_r\) as:
\begin{equation*}
    \bm{v}^n_r = \begin{bmatrix}
        G * \left(-(\nabla \delta f^n)_y + (\delta f^n_{b})_y\right)\\
        G * \left((\nabla \delta f^n)_x - (\delta f^n_{b})_x\right)
    \end{bmatrix},
\end{equation*}  
where \(G\) represents the Gaussian blur operator, used to ensure that \(\bm{v}^n_r\) varies smoothly across each pixel within a patch, making it more reflective of real-world scenarios.

\section{Experimental Results}

\subsection{Tiny Object Detection on UAVDB}
\label{ssec:appendix_uavdb}

\begin{table*}
    % \small
    \centering
    % \resizebox{!}{\lineheight}{ % Adjust the table to the width of the page
    \begin{adjustbox}{max width=\textwidth, max height=0.5\textheight}
    \begin{tabular}{cccccccccc}
        \toprule
        \multirow{2}{*}{Methods} & \multirow{2}{*}{Model} & Training Time & Inference Time & \#Param. & FLOPs & \multirow{2}{*}{$\text{AP}^{val}_{50}$} & \multirow{2}{*}{$\text{AP}^{val}_{50-95}$} & \multirow{2}{*}{$\text{AP}^{test}_{50}$} & \multirow{2}{*}{$\text{AP}^{test}_{50-95}$}\\
            & & (hours:mins:sec) & (per image, ms) & (M) & (G) & \\
        \midrule
        \multirow{5}{*}{RGB} & YOLO11n & 01:00:24 & 0.8 & 2.6 & 6.3 & 0.849 & 0.549 & 0.811 & 0.518 \\
        & YOLO11s & 01:07:58 & 0.8 & 9.4 & 21.3 & 0.844 & 0.559 & 0.837 & \textbf{0.558} \\
        & YOLO11m & 01:42:09 & 1.0 & 20.0 & 67.6 & 0.869 & 0.583 & \textbf{0.856} & 0.546 \\
        & YOLO11l & 02:17:13 & 1.2 & 25.3 & 86.6 & 0.840 & 0.580 & 0.812 & 0.557 \\
        & YOLO11x & 02:50:47 & 1.6 & 56.8 & 194.4 & 0.867 & 0.583 & 0.781 & 0.520 \\
        \midrule
        \multirow{5}{*}{Grayscale} & YOLO11n & 00:58:40 & 0.7 & 2.6 & 6.3 & 0.770 & 0.338 & 0.660 & 0.281 \\
        & YOLO11s & 01:09:01 & 0.8 & 9.4 & 21.3 & 0.747 & 0.329 & 0.606 & 0.263 \\
        & YOLO11m & 01:42:17 & 1.1 & 20.0 & 67.6 & 0.753 & 0.334 & 0.697 & 0.320 \\
        & YOLO11l & 02:14:29 & 1.3 & 25.3 & 86.6 & 0.738 & 0.325 & 0.748 & 0.339 \\
        & YOLO11x & 02:51:36 & 1.6 & 56.8 & 194.4 & 0.736 & 0.319 & 0.729 & 0.331 \\
        \bottomrule
    \end{tabular}
    % }
    \end{adjustbox}
    \caption{YOLO11 performance comparison on UAVDB with RGB and Grayscale inputs.}
    \label{tab:experiments_uavdb_rgb_grayscale}
\end{table*}

\begin{table*}
    % \small
    \centering
    % \resizebox{!}{\lineheight}{ % Adjust the table to the width of the page
    \begin{adjustbox}{max width=\textwidth, max height=0.5\textheight}
    \begin{tabular}{cccccccccc}
        \toprule
        \multirow{2}{*}{Methods} & \multirow{2}{*}{Model} & Training Time & Inference Time & \#Param. & FLOPs & \multirow{2}{*}{$\text{AP}^{val}_{50}$} & \multirow{2}{*}{$\text{AP}^{val}_{50-95}$} & \multirow{2}{*}{$\text{AP}^{test}_{50}$} & \multirow{2}{*}{$\text{AP}^{test}_{50-95}$}\\
            & & (hours:mins:sec) & (per image, ms) & (M) & (G) & \\
        \midrule
        \multirow{5}{*}{Horn-Schunck~\cite{horn1981determining}} & YOLO11n & 00:57:07 & 0.4 & 2.6 & 6.3 & 0.062 & 0.021 & 0.104 & 0.021 \\
        & YOLO11s & 01:05:49 & 0.8 & 9.4 & 21.3 & 0.038 & 0.013 & 0.012 & 0.003 \\
        & YOLO11m & 01:39:02 & 1.1 & 20.0 & 67.6 & 0.037 & 0.012 & 0.021 & 0.006 \\
        & YOLO11l & 02:11:58 & 0.9 & 25.3 & 86.6 & 0.002 & 0.000 & 0.000 & 0.000 \\
        & YOLO11x & 02:47:02 & 1.6 & 56.8 & 194.4 & 0.027 & 0.008 & 0.025 & 0.008 \\
        \midrule
        \multirow{5}{*}{Lucas-Kanade~\cite{lucas1981iterative}} & YOLO11n & 00:58:23 & 0.5 & 2.6 & 6.3 & 0.253 & 0.152 & 0.500 & 0.200 \\
        & YOLO11s & 01:07:00 & 0.6 & 9.4 & 21.3 & 0.122 & 0.054 & 0.038 & 0.015 \\
        & YOLO11m & 01:39:56 & 0.9 & 20.0 & 67.6 & 0.051 & 0.019 & 0.029 & 0.012 \\
        & YOLO11l & 02:16:21 & 1.0 & 25.3 & 86.6 & 0.138 & 0.070 & 0.048 & 0.018 \\
        & YOLO11x & 02:51:06 & 1.6 & 56.8 & 194.4 & 0.033 & 0.015 & 0.008 & 0.004 \\
        \midrule
        \multirow{5}{*}{Farneback~\cite{farneback2003two}} & YOLO11n & 00:57:24 & 0.4 & 2.6 & 6.3 & 0.465 & 0.264 & 0.258 & 0.145 \\
        & YOLO11s & 01:07:18 & 0.7 & 9.4 & 21.3 & 0.450 & 0.242 & 0.205 & 0.098 \\
        & YOLO11m & 01:39:13 & 0.8 & 20.0 & 67.6 & 0.460 & 0.207 & 0.174 & 0.094 \\
        & YOLO11l & 02:13:39 & 1.1 & 25.3 & 86.6 & 0.505 & 0.210 & 0.254 & 0.123 \\
        & YOLO11x & 02:48:12 & 1.5 & 56.8 & 194.4 & 0.408 & 0.209 & 0.203 & 0.094 \\
        \midrule
        \multirow{5}{*}{Brox~\cite{brox2004high}} & YOLO11n & 00:58:25 & 0.7 & 2.6 & 6.3 & 0.454 & 0.218 & 0.244 & 0.110 \\
        & YOLO11s & 01:07:09 & 0.8 & 9.4 & 21.3 & 0.428 & 0.211 & 0.214 & 0.095 \\
        & YOLO11m & 01:39:40 & 1.0 & 20.0 & 67.6 & 0.429 & 0.213 & 0.218 & 0.097 \\
        & YOLO11l & 02:13:53 & 1.3 & 25.3 & 86.6 & 0.422 & 0.214 & 0.180 & 0.074 \\
        & YOLO11x & 02:49:54 & 1.6 & 56.8 & 194.4 & 0.401 & 0.189 & 0.190 & 0.082 \\
        \midrule
        \multirow{5}{*}{TV-L1~\cite{zach2007duality}} & YOLO11n & 00:58:19 & 0.7 & 2.6 & 6.3 & 0.719 & 0.364 & \textbf{0.779} & 0.409 \\
        & YOLO11s & 01:07:24 & 0.7 & 9.4 & 21.3 & 0.715 & 0.376 & 0.775 & 0.411 \\
        & YOLO11m & 01:40:50 & 1.1 & 20.0 & 67.6 & 0.759 & 0.393 & 0.782 & \textbf{0.431} \\
        & YOLO11l & 02:17:32 & 1.3 & 25.3 & 86.6 & 0.742 & 0.401 & 0.763 & 0.416 \\
        & YOLO11x & 02:48:50 & 1.6 & 56.8 & 194.4 & 0.767 & 0.396 & 0.781 & 0.387 \\
        \midrule
        \multirow{5}{*}{SimpleFlow~\cite{tao2012simpleflow}} & YOLO11n &  &  & 2.6 & 6.3 & 0. & 0. & 0. & 0. \\
        & YOLO11s &  &  & 9.4 & 21.3 & 0. & 0. & 0. & 0. \\
        & YOLO11m &  &  & 20.0 & 67.6 & 0. & 0. & 0. & 0. \\
        & YOLO11l &  &  & 25.3 & 86.6 & 0. & 0. & 0. & 0. \\
        & YOLO11x &  &  & 56.8 & 194.4 & 0. & 0. & 0. & 0. \\
        \midrule
        \multirow{5}{*}{RLOF~\cite{senst2012robust}} & YOLO11n & 00:57:10 & 0.6 & 2.6 & 6.3 & 0.172 & 0.079 & 0.097 & 0.039 \\
        & YOLO11s & 01:08:03 & 0.8 & 9.4 & 21.3 & 0.183 & 0.087 & 0.091 & 0.039 \\
        & YOLO11m & 01:42:02 & 1.1 & 20.0 & 67.6 & 0.180 & 0.088 & 0.110 & 0.050 \\
        & YOLO11l & 02:14:07 & 1.3 & 25.3 & 86.6 & 0.181 & 0.090 & 0.124 & 0.055 \\
        & YOLO11x & 02:51:59 & 1.6 & 56.8 & 194.4 & 0.180 & 0.087 & 0.105 & 0.047 \\
        \midrule
        \multirow{5}{*}{DeepFlow~\cite{weinzaepfel2013deepflow}} & YOLO11n & 01:01:37 & 0.7 & 2.6 & 6.3 & 0.118 & 0.050 & 0.154 & 0.058 \\
        & YOLO11s & 01:10:16 & 0.8 & 9.4 & 21.3 & 0.122 & 0.051 & 0.150 & 0.059 \\
        & YOLO11m & 01:43:47 & 1.1 & 20.0 & 67.6 & 0.123 & 0.052 & 0.156 & 0.061 \\
        & YOLO11l & 02:16:42 & 1.3 & 25.3 & 86.6 & 0.129 & 0.052 & 0.162 & 0.062 \\
        & YOLO11x & 02:54:47 & 1.6 & 56.8 & 194.4 & 0.132 & 0.055 & 0.163 & 0.063 \\
        \midrule
        \multirow{5}{*}{PCAFlow~\cite{wulff2015efficient}} & YOLO11n & 00:58:31 & 0.7 & 2.6 & 6.3 & 0.399 & 0.235 & 0.547 & 0.332 \\
        & YOLO11s & 01:08:27 & 0.8 & 9.4 & 21.3 & 0.413 & 0.252 & 0.547 & 0.332 \\
        & YOLO11m & 01:42:02 & 1.2 & 20.0 & 67.6 & 0.418 & 0.249 & 0.557 & 0.313 \\
        & YOLO11l & 02:17:19 & 1.3 & 25.3 & 86.6 & 0.416 & 0.253 & 0.525 & 0.326 \\
        & YOLO11x & 02:51:27 & 1.6 & 56.8 & 194.4 & 0.425 & 0.255 & 0.591 & 0.353 \\
        \midrule
        \multirow{5}{*}{DIS~\cite{kroeger2016fast}} & YOLO11n & 00:58:58 & 0.7 & 2.6 & 6.3 & 0.345 & 0.149 & 0.151 & 0.057 \\
        & YOLO11s & 01:08:51 & 0.8 & 9.4 & 21.3 & 0.336 & 0.149 & 0.149 & 0.056 \\
        & YOLO11m & 01:40:38 & 1.1 & 20.0 & 67.6 & 0.322 & 0.149 & 0.119 & 0.048 \\
        & YOLO11l & 02:16:17 & 1.3 & 25.3 & 86.6 & 0.358 & 0.158 & 0.153 & 0.060 \\
        & YOLO11x & 02:49:32 & 1.6 & 56.8 & 194.4 & 0.367 & 0.164 & 0.136 & 0.052 \\
        \midrule
        \multirow{5}{*}{\textbf{ReynoldsFlow (ours)}} & YOLO11n & 00:59:54 & 0.5 & 2.6 & 6.3 & 0.500 & 0.325 & 0.500 & 0.288 \\
        & YOLO11s & 01:08:42 & 0.6 & 9.4 & 21.3 & 0.493 & 0.282 & 0.666 & 0.370 \\
        & YOLO11m & 01:41:26 & 1.0 & 20.0 & 67.6 & 0.536 & 0.319 & 0.762 & 0.421 \\
        & YOLO11l & 02:15:58 & 1.3 & 25.3 & 86.6 & 0.528 & 0.304 & 0.722 & 0.335 \\
        & YOLO11x & 02:50:56 & 1.3 & 56.8 & 194.4 & 0.509 & 0.347 & 0.443 & 0.225 \\
        \bottomrule
    \end{tabular}
    % }
    \end{adjustbox}
    \caption{YOLO11 performance comparison on UAVDB across optical flow methods in HSV space visualization.}
    \label{tab:experiments_uavdb_hsv}
\end{table*}

\begin{table*}
    % \small
    \centering
    % \resizebox{!}{\lineheight}{ % Adjust the table to the width of the page
    \begin{adjustbox}{max width=\textwidth, max height=0.5\textheight}
    \begin{tabular}{cccccccccc}
        \toprule
        \multirow{2}{*}{Methods} & \multirow{2}{*}{Model} & Training Time & Inference Time & \#Param. & FLOPs & \multirow{2}{*}{$\text{AP}^{val}_{50}$} & \multirow{2}{*}{$\text{AP}^{val}_{50-95}$} & \multirow{2}{*}{$\text{AP}^{test}_{50}$} & \multirow{2}{*}{$\text{AP}^{test}_{50-95}$}\\
            & & (hours:mins:sec) & (per image, ms) & (M) & (G) & \\
        \midrule
        \multirow{5}{*}{Horn-Schunck~\cite{horn1981determining}} & YOLO11n & 00:59:17 & 0.6 & 2.6 & 6.3 & 0.507 & 0.253 & 0.633 & 0.311 \\
        & YOLO11s & 01:08:39 & 0.7 & 9.4 & 21.3 & 0.472 & 0.236 & 0.652 & 0.313 \\
        & YOLO11m & 01:40:34 & 1.0 & 20.0 & 67.6 & 0.479 & 0.243 & 0.696 & 0.345 \\
        & YOLO11l & 02:14:24 & 1.3 & 25.3 & 86.6 & 0.451 & 0.220 & 0.613 & 0.295 \\
        & YOLO11x & 02:49:14 & 1.6 & 56.8 & 194.4 & 0.465 & 0.235 & 0.663 & 0.328 \\
        \midrule
        \multirow{5}{*}{Lucas-Kanade~\cite{lucas1981iterative}} & YOLO11n & 01:21:25 & 1.1 & 2.6 & 6.3 & 0.539 & 0.295 & 0.208 & 0.104 \\
        & YOLO11s & 01:23:11 & 1.2 & 9.4 & 21.3 & 0.580 & 0.323 & 0.236 & 0.115 \\
        & YOLO11m & 01:46:40 & 1.6 & 20.0 & 67.6 & 0.579 & 0.330 & 0.208 & 0.104 \\
        & YOLO11l & 02:19:01 & 1.8 & 25.3 & 86.6 & 0.594 & 0.324 & 0.220 & 0.108 \\
        & YOLO11x & 02:54:26 & 2.1 & 56.8 & 194.4 & 0.604 & 0.327 & 0.241 & 0.122 \\
        \midrule
        \multirow{5}{*}{Farneback~\cite{farneback2003two}} & YOLO11n & 00:58:33 & 0.7 & 2.6 & 6.3 & 0.840 & 0.547 & 0.682 & 0.444 \\
        & YOLO11s & 01:08:52 & 0.7 & 9.4 & 21.3 & 0.857 & 0.556 & 0.674 & 0.434 \\
        & YOLO11m & 01:40:49 & 1.1 & 20.0 & 67.6 & 0.841 & 0.548 & 0.693 & 0.446 \\
        & YOLO11l & 02:16:56 & 1.3 & 25.3 & 86.6 & 0.858 & 0.552 & 0.667 & 0.436 \\
        & YOLO11x & 02:48:47 & 1.6 & 56.8 & 194.4 & 0.843 & 0.546 & 0.719 & 0.481 \\
        \midrule
        \multirow{5}{*}{Brox~\cite{brox2004high}} & YOLO11n & 01:09:32 & 0.9 & 2.6 & 6.3 & 0.669 & 0.344 & 0.371 & 0.172 \\
        & YOLO11s & 01:12:16 & 1.0 & 9.4 & 21.3 & 0.672 & 0.350 & 0.362 & 0.173 \\
        & YOLO11m & 01:41:41 & 1.4 & 20.0 & 67.6 & 0.696 & 0.365 & 0.397 & 0.191 \\
        & YOLO11l & 02:16:09 & 1.5 & 25.3 & 86.6 & 0.698 & 0.363 & 0.413 & 0.197 \\
        & YOLO11x & 02:50:11 & 1.8 & 56.8 & 194.4 & 0.694 & 0.359 & 0.397 & 0.194 \\
        \midrule
        \multirow{5}{*}{TV-L1~\cite{zach2007duality}} & YOLO11n & 00:58:33 & 0.7 & 2.6 & 6.3 & 0.814 & 0.430 & 0.696 & 0.376 \\
        & YOLO11s & 01:07:53 & 0.7 & 9.4 & 21.3 & 0.814 & 0.435 & 0.705 & 0.403 \\
        & YOLO11m & 01:41:49 & 1.0 & 20.0 & 67.6 & 0.792 & 0.435 & 0.774 & 0.456 \\
        & YOLO11l & 02:14:29 & 1.3 & 25.3 & 86.6 & 0.820 & 0.451 & 0.748 & 0.431 \\
        & YOLO11x & 02:51:57 & 1.6 & 56.8 & 194.4 & 0.810 & 0.458 & 0.719 & 0.418 \\
        \midrule
        \multirow{5}{*}{SimpleFlow~\cite{tao2012simpleflow}} & YOLO11n &  &  & 2.6 & 6.3 & 0. & 0. & 0. & 0. \\
        & YOLO11s &  &  & 9.4 & 21.3 & 0. & 0. & 0. & 0. \\
        & YOLO11m &  &  & 20.0 & 67.6 & 0. & 0. & 0. & 0. \\
        & YOLO11l &  &  & 25.3 & 86.6 & 0. & 0. & 0. & 0. \\
        & YOLO11x &  &  & 56.8 & 194.4 & 0. & 0. & 0. & 0. \\
        \midrule
        \multirow{5}{*}{RLOF~\cite{senst2012robust}} & YOLO11n & 00:58:52 & 0.7 & 2.6 & 6.3 & 0.369 & 0.173 & 0.339 & 0.152 \\
        & YOLO11s & 01:06:55 & 0.8 & 9.4 & 21.3 & 0.360 & 0.170 & 0.337 & 0.146 \\
        & YOLO11m & 01:39:21 & 1.1 & 20.0 & 67.6 & 0.352 & 0.172 & 0.361 & 0.166 \\
        & YOLO11l & 02:14:01 & 1.3 & 25.3 & 86.6 & 0.354 & 0.170 & 0.375 & 0.172 \\
        & YOLO11x & 02:52:35 & 1.6 & 56.8 & 194.4 & 0.351 & 0.168 & 0.356 & 0.153 \\
        \midrule
        \multirow{5}{*}{DeepFlow~\cite{weinzaepfel2013deepflow}} & YOLO11n & 01:00:42 & 0.7 & 2.6 & 6.3 & 0.462 & 0.214 & 0.670 & 0.309 \\
        & YOLO11s & 01:09:31 & 0.8 & 9.4 & 21.3 & 0.478 & 0.221 & 0.663 & 0.309 \\
        & YOLO11m & 01:42:02 & 1.0 & 20.0 & 67.6 & 0.483 & 0.232 & 0.684 & 0.328 \\
        & YOLO11l & 02:16:08 & 1.3 & 25.3 & 86.6 & 0.441 & 0.201 & 0.702 & 0.340 \\
        & YOLO11x & 02:52:55 & 1.6 & 56.8 & 194.4 & 0.456 & 0.211 & 0.637 & 0.304 \\
        \midrule
        \multirow{5}{*}{PCAFlow~\cite{wulff2015efficient}}& YOLO11n & 00:58:47 & 0.7 & 2.6 & 6.3 & 0.492 & 0.247 & 0.657 & 0.328 \\
        & YOLO11s & 01:08:45 & 0.8 & 9.4 & 21.3 & 0.492 & 0.248 & 0.563 & 0.273 \\
        & YOLO11m & 01:42:26 & 1.1 & 20.0 & 67.6 & 0.498 & 0.241 & 0.674 & 0.342 \\
        & YOLO11l & 02:17:00 & 1.3 & 25.3 & 86.6 & 0.488 & 0.248 & 0.628 & 0.308 \\
        & YOLO11x & 02:50:41 & 1.6 & 56.8 & 194.4 & 0.457 & 0.229 & 0.665 & 0.328 \\
        \midrule
        \multirow{5}{*}{DIS~\cite{kroeger2016fast}} & YOLO11n & 01:01:05 & 0.9 & 2.6 & 6.3 & 0.435 & 0.199 & 0.555 & 0.260 \\
        & YOLO11s & 01:09:41 & 0.9 & 9.4 & 21.3 & 0.438 & 0.214 & 0.540 & 0.258 \\
        & YOLO11m & 01:42:19 & 1.1 & 20.0 & 67.6 & 0.444 & 0.215 & 0.597 & 0.286 \\
        & YOLO11l & 02:17:23 & 1.3 & 25.3 & 86.6 & 0.475 & 0.227 & 0.580 & 0.285 \\
        & YOLO11x & 02:51:21 & 1.6 & 56.8 & 194.4 & 0.479 & 0.234 & 0.611 & 0.304 \\
        \midrule
        \multirow{5}{*}{\textbf{ReynoldsFlow (ours)}} & YOLO11n & 00:58:31 & 0.6 & 2.6 & 6.3 & 0.910 & 0.571 & 0.895 & 0.547 \\
        & YOLO11s & 01:07:09 & 0.7 & 9.4 & 21.3 & 0.900 & 0.567 & \textbf{0.906} & 0.535 \\
        & YOLO11m & 01:39:57 & 1.1 & 20.0 & 67.6 & 0.909 & 0.572 & 0.893 & 0.573 \\
        & YOLO11l & 02:14:01 & 1.3 & 25.3 & 86.6 & 0.899 & 0.576 & 0.904 & \textbf{0.596} \\
        & YOLO11x & 02:51:50 & 1.6 & 56.8 & 194.4 & 0.902 & 0.569 & 0.831 & 0.507 \\
        \bottomrule
    \end{tabular}
    % }
    \end{adjustbox}
    \caption{YOLO11 performance comparison on UAVDB across optical flow methods with enhanced flow visualization.}
    \label{tab:experiments_uavdb_mag}
\end{table*}

\subsection{Pose Estimation on GolfDB}
\label{ssec:appendix_golfdb}

\begin{table}
    \centering
    \begin{adjustbox}{max width=\linewidth}
    \begin{tabular}{cccccc}
        \toprule
        \multirow{2}{*}{Methods} & \multirow{2}{*}{Split} & Training Time & \multirow{2}{*}{Average Loss} & \multirow{2}{*}{PCE}\\
            & & (hours:mins:sec) & & \\
        \midrule
        \multirow{4}{*}{RGB} & 1 & 00:08:37 & 0.2354 & 0.708 \\
            & 2 & 00:08:29 & 0.2275 & 0.688 \\
            & 3 & 00:08:08 & 0.2289 & 0.715 \\
            & 4 & 00:08:19 & 0.2334 & 0.708 \\
        \midrule
        \multirow{4}{*}{Grayscale} & 1 & 00:08:35 & 0.2496 & 0.711 \\
        & 2 & 00:08:27 & 0.2435 & 0.679 \\
        & 3 & 00:07:59 & 0.2432 & 0.699 \\
        & 4 & 00:08:22 & 0.2542 & 0.703 \\
        \bottomrule
    \end{tabular}
    \end{adjustbox}
    \caption{SwingNet performance comparison on GolfDB with RGB and Grayscale inputs.}
    \label{tab:experiments_golfdb_rgb_grayscale}
\end{table}

\begin{table}
    % \small
    \centering
    \resizebox{\linewidth}{!}{ % Adjust table to the width of the page
    \begin{tabular}{cccccc}
        \toprule
        \multirow{2}{*}{Methods} & \multirow{2}{*}{Split} & Training Time & \multirow{2}{*}{Average Loss} & \multirow{2}{*}{PCE}\\
         & & (hours:mins:sec) & & \\
        \midrule
        \multirow{4}{*}{Horn-Schunck~\cite{horn1981determining}} & 1 &  &  &  \\
        & 2 &  &  &  \\
        & 3 &  &  &  \\
        & 4 &  &  &  \\
        \midrule
        \multirow{4}{*}{Lucas-Kanade~\cite{lucas1981iterative}} & 1 &  &  &  \\
        & 2 &  &  &  \\
        & 3 &  &  &  \\
        & 4 &  &  &  \\
        \midrule
        \multirow{4}{*}{Farneback~\cite{farneback2003two}} & 1 &  &  &  \\
        & 2 &  &  &  \\
        & 3 &  &  &  \\
        & 4 &  &  &  \\
        \midrule
        \multirow{4}{*}{Brox~\cite{brox2004high}} & 1 &  &  &  \\
        & 2 &  &  &  \\
        & 3 &  &  &  \\
        & 4 &  &  &  \\
        \midrule
        \multirow{4}{*}{TV-L1~\cite{zach2007duality}} & 1 &  &  &  \\
        & 2 &  &  &  \\
        & 3 &  &  &  \\
        & 4 &  &  &  \\
        \midrule
        \multirow{4}{*}{SimpleFlow~\cite{tao2012simpleflow}} & 1 &  &  &  \\
        & 2 &  &  &  \\
        & 3 &  &  &  \\
        & 4 &  &  &  \\
        \midrule
        \multirow{4}{*}{RLOF~\cite{senst2012robust}} & 1 &  &  &  \\
        & 2 &  &  &  \\
        & 3 &  &  &  \\
        & 4 &  &  &  \\
        \midrule
        \multirow{4}{*}{DeepFlow~\cite{weinzaepfel2013deepflow}} & 1 &  &  &  \\
        & 2 &  &  &  \\
        & 3 &  &  &  \\
        & 4 &  &  &  \\
        \midrule
        \multirow{4}{*}{PCAFlow~\cite{wulff2015efficient}} & 1 &  &  &  \\
        & 2 &  &  &  \\
        & 3 &  &  &  \\
        & 4 &  &  &  \\
        \midrule
        \multirow{4}{*}{DIS~\cite{kroeger2016fast}} & 1 &  &  &  \\
        & 2 &  &  &  \\
        & 3 &  &  &  \\
        & 4 &  &  &  \\
        \midrule
        \multirow{4}{*}{\textbf{ReynoldsFlow (ours)}} & 1 & & & \\
        & 2 &  &  &  \\
        & 3 &  &  &  \\
        & 4 &  &  &  \\
        \bottomrule
    \end{tabular}
 }
    \caption{SwingNet performance comparison on GolfDB across optical flow methods in HSV space visualization.}
    \label{tab:experiments_golfdb_hsv}
\end{table}

\begin{table}
    % \small
    \centering
    \resizebox{\linewidth}{!}{ % Adjust table to the width of the page
    \begin{tabular}{cccccc}
        \toprule
        \multirow{2}{*}{Methods} & \multirow{2}{*}{Split} & Training Time & \multirow{2}{*}{Average Loss} & \multirow{2}{*}{PCE}\\
         & & (hours:mins:sec) & & \\
        \midrule
        \multirow{4}{*}{Horn-Schunck~\cite{horn1981determining}} & 1 & 00:08:36 & 0.2012 & 0.762 \\
        & 2 & 00:08:19 & 0.1913 & 0.740\\
        & 3 & 00:08:02 & 0.1895 & 0.741\\
        & 4 & 00:08:20 & 0.2023 & 0.760\\
        \midrule
        \multirow{4}{*}{Lucas-Kanade~\cite{lucas1981iterative}} & 1 & 00:08:33 & 0.2179 & 0.759\\
        & 2 & 00:08:20 & 0.2010 & 0.729\\
        & 3 & 00:08:03 & 0.2012 & 0.737\\
        & 4 & 00:08:19 & 0.2085 & 0.743\\
        \midrule
        \multirow{4}{*}{Farneback~\cite{farneback2003two}} & 1 & 00:08:31 & 0.2169 & 0.755\\
        & 2 & 00:08:34 & 0.2122 & 0.751\\
        & 3 & 00:08:02 & 0.2116 & 0.762\\
        & 4 & 00:08:19 & 0.2100 & 0.750\\
        \midrule
        \multirow{4}{*}{Brox~\cite{brox2004high}} & 1 & 00:08:33 & 0.2351 & 0.727\\
        & 2 & 00:08:19 & 0.2228 & 0.717\\
        & 3 & 00:08:03 & 0.2197 & 0.710\\
        & 4 & 00:08:19 & 0.2257 & 0.725\\
        \midrule
        \multirow{4}{*}{TV-L1~\cite{zach2007duality}} & 1 & 00:08:44 & 0.1715 & 0.795\\
        & 2 & 00:08:36 & 0.1725 & 0.791\\
        & 3 & 00:08:04 & 0.1679 & 0.786\\
        & 4 & 00:08:27 & 0.1666 & 0.792\\
        \midrule
        \multirow{4}{*}{SimpleFlow~\cite{tao2012simpleflow}} & 1 & 00:08:33 & 0.2638 & 0.644\\
        & 2 & 00:08:20 & 0.2660 & 0.655\\
        & 3 & 00:08:03 & 0.2695 & 0.644\\
        & 4 & 00:08:10 & 0.2651 & 0.653\\
        \midrule
        \multirow{4}{*}{RLOF~\cite{senst2012robust}} & 1 & 00:08:42 & 0.2930 & 0.611\\
        & 2 & 00:08:36 & 0.2754 & 0.588\\
        & 3 & 00:08:05 & 0.2917 & 0.613\\
        & 4 & 00:08:23 & 0.2906 & 0.605\\
        \midrule
        \multirow{4}{*}{DeepFlow~\cite{weinzaepfel2013deepflow}} & 1 & 00:08:33 & 0.2445 & 0.693\\
        & 2 & 00:08:19 & 0.2239 & 0.671\\
        & 3 & 00:08:22 & 0.2380 & 0.667\\
        & 4 & 00:08:20 & 0.2305 & 0.667\\
        \midrule
        \multirow{4}{*}{PCAFlow~\cite{wulff2015efficient}} & 1 & 00:08:43 & 0.2169 & 0.713\\
        & 2 & 00:08:36 & 0.2136 & 0.718\\
        & 3 & 00:08:28 & 0.2136 & 0.709\\
        & 4 & 00:08:16 & 0.2150 & 0.702\\
        \midrule
        \multirow{4}{*}{DIS~\cite{kroeger2016fast}} & 1 & 00:08:33 & 0.2044 & 0.766\\
        & 2 & 00:08:19 & 0.1950 & 0.772\\
        & 3 & 00:08:14 & 0.1990 & 0.754\\
        & 4 & 00:08:21 & 0.2003 & 0.754\\
        \midrule
        \multirow{4}{*}{\textbf{ReynoldsFlow (ours)}} & 1 & 00:08:24 & \textbf{0.1695} & \textbf{0.799} \\
        & 2 & 00:08:40 & \textbf{0.1674} & \textbf{0.803} \\
        & 3 & 00:08:48 & \textbf{0.1599} & \textbf{0.793} \\
        & 4 & 00:08:56 & \textbf{0.1722} & \textbf{0.801} \\
        \bottomrule
    \end{tabular}
    }
    \caption{SwingNet performance comparison on GolfDB across optical flow methods with enhanced flow visualization.}
    \label{tab:experiments_golfdb_enhanced}
\end{table}

\begin{figure*}[tp]
    \centering
    \includegraphics[width=0.8\linewidth]{}
    \caption{A detailed comparison of the two visualization approaches for each optical flow method is provided for two scenarios: frames 950 and 951 from Camera 0 in Dataset 1 and frames 1300 and 1301 from Camera 0 in Dataset 3.}
    \label{fig:appendix_fig1}
\end{figure*}

\begin{figure*}[tp]
    \centering
    \includegraphics[width=\linewidth]{figs/appendix_fig2.jpg}
    \caption{.}
    \label{fig:appendix_fig2}
\end{figure*}
