# Supplementary material for: ReynoldsFlow: Physics-Inspired Spatiotemporal Flow Representation for Video Understanding
Source: arXiv:2503.04500 source file (2026-08-20)
Supplement: Supplementary file 2 [file X_suppl.tex]

% \clearpage
% \setcounter{page}{1}
\maketitlesupplementary

\begin{table*}
    % \small
    \centering
    % \resizebox{!}{\lineheight}{ % Adjust the table to the width of the page
    \begin{adjustbox}{max width=\textwidth, max height=0.5\textheight}
    \begin{tabular}{cccccccccc}
        \toprule
        \multirow{2}{*}{Methods} & \multirow{2}{*}{Model} & Training Time & Inference Time & \#Param. & FLOPs & \multirow{2}{*}{$\text{AP}^{val}_{50}$} & \multirow{2}{*}{$\text{AP}^{val}_{50-95}$} & \multirow{2}{*}{$\text{AP}^{test}_{50}$} & \multirow{2}{*}{$\text{AP}^{test}_{50-95}$}\\
            & & (hours:mins:sec) & (per image, ms) & (M) & (G) & \\
        \midrule
        \multirow{5}{*}{Horn-Schunck~\cite{horn1981determining}} & YOLO11n & 00:57:07 & 0.4 & 2.6 & 6.3 & 0.062 & 0.021 & 0.104 & 0.021 \\
        & YOLO11s & 01:05:49 & 0.8 & 9.4 & 21.3 & 0.038 & 0.013 & 0.012 & 0.003 \\
        & YOLO11m & 01:39:02 & 1.1 & 20.0 & 67.6 & 0.037 & 0.012 & 0.021 & 0.006 \\
        & YOLO11l & 02:11:58 & 0.9 & 25.3 & 86.6 & 0.002 & 0.000 & 0.000 & 0.000 \\
        & YOLO11x & 02:47:02 & 1.6 & 56.8 & 194.4 & 0.027 & 0.008 & 0.025 & 0.008 \\
        \midrule
        \multirow{5}{*}{Lucas-Kanade~\cite{lucas1981iterative}} & YOLO11n & 00:58:23 & 0.5 & 2.6 & 6.3 & 0.253 & 0.152 & 0.500 & 0.200 \\
        & YOLO11s & 01:07:00 & 0.6 & 9.4 & 21.3 & 0.122 & 0.054 & 0.038 & 0.015 \\
        & YOLO11m & 01:39:56 & 0.9 & 20.0 & 67.6 & 0.051 & 0.019 & 0.029 & 0.012 \\
        & YOLO11l & 02:16:21 & 1.0 & 25.3 & 86.6 & 0.138 & 0.070 & 0.048 & 0.018 \\
        & YOLO11x & 02:51:06 & 1.6 & 56.8 & 194.4 & 0.033 & 0.015 & 0.008 & 0.004 \\
        \midrule
        \multirow{5}{*}{Farneback~\cite{farneback2003two}} & YOLO11n & 00:57:24 & 0.4 & 2.6 & 6.3 & 0.465 & 0.264 & 0.258 & 0.145 \\
        & YOLO11s & 01:07:18 & 0.7 & 9.4 & 21.3 & 0.450 & 0.242 & 0.205 & 0.098 \\
        & YOLO11m & 01:39:13 & 0.8 & 20.0 & 67.6 & 0.460 & 0.207 & 0.174 & 0.094 \\
        & YOLO11l & 02:13:39 & 1.1 & 25.3 & 86.6 & 0.505 & 0.210 & 0.254 & 0.123 \\
        & YOLO11x & 02:48:12 & 1.5 & 56.8 & 194.4 & 0.408 & 0.209 & 0.203 & 0.094 \\
        \midrule
        \multirow{5}{*}{Brox~\cite{brox2004high}} & YOLO11n & 00:58:25 & 0.7 & 2.6 & 6.3 & 0.454 & 0.218 & 0.244 & 0.110 \\
        & YOLO11s & 01:07:09 & 0.8 & 9.4 & 21.3 & 0.428 & 0.211 & 0.214 & 0.095 \\
        & YOLO11m & 01:39:40 & 1.0 & 20.0 & 67.6 & 0.429 & 0.213 & 0.218 & 0.097 \\
        & YOLO11l & 02:13:53 & 1.3 & 25.3 & 86.6 & 0.422 & 0.214 & 0.180 & 0.074 \\
        & YOLO11x & 02:49:54 & 1.6 & 56.8 & 194.4 & 0.401 & 0.189 & 0.190 & 0.082 \\
        \midrule
        \multirow{5}{*}{TV-L1~\cite{zach2007duality}} & YOLO11n & 00:58:19 & 0.7 & 2.6 & 6.3 & 0.719 & 0.364 & \textbf{0.779} & 0.409 \\
        & YOLO11s & 01:07:24 & 0.7 & 9.4 & 21.3 & 0.715 & 0.376 & 0.775 & 0.411 \\
        & YOLO11m & 01:40:50 & 1.1 & 20.0 & 67.6 & 0.759 & 0.393 & 0.782 & \textbf{0.431} \\
        & YOLO11l & 02:17:32 & 1.3 & 25.3 & 86.6 & 0.742 & 0.401 & 0.763 & 0.416 \\
        & YOLO11x & 02:48:50 & 1.6 & 56.8 & 194.4 & 0.767 & 0.396 & 0.781 & 0.387 \\
        \midrule
        \multirow{5}{*}{SimpleFlow~\cite{tao2012simpleflow}} & YOLO11n & 00:55:43 & 0.6 & 2.6 & 6.3 & 0.566 & 0.338 & 0.444 & 0.250 \\
        & YOLO11s & 01:05:51 & 0.7 & 9.4 & 21.3 & 0.560 & 0.329 & 0.414 & 0.234 \\
        & YOLO11m & 01:37:25 & 1.1 & 20.0 & 67.6 & 0.578 & 0.340 & 0.456 & 0.262 \\
        & YOLO11l & 02:12:42 & 1.3 & 25.3 & 86.6 & 0.552 & 0.313 & 0.471 & 0.255 \\
        & YOLO11x & 02:46:57 & 1.6 & 56.8 & 194.4 & 0.554 & 0.322 & 0.444 & 0.251 \\
        \midrule
        \multirow{5}{*}{RLOF~\cite{senst2012robust}} & YOLO11n & 00:57:10 & 0.6 & 2.6 & 6.3 & 0.172 & 0.079 & 0.097 & 0.039 \\
        & YOLO11s & 01:08:03 & 0.8 & 9.4 & 21.3 & 0.183 & 0.087 & 0.091 & 0.039 \\
        & YOLO11m & 01:42:02 & 1.1 & 20.0 & 67.6 & 0.180 & 0.088 & 0.110 & 0.050 \\
        & YOLO11l & 02:14:07 & 1.3 & 25.3 & 86.6 & 0.181 & 0.090 & 0.124 & 0.055 \\
        & YOLO11x & 02:51:59 & 1.6 & 56.8 & 194.4 & 0.180 & 0.087 & 0.105 & 0.047 \\
        \midrule
        \multirow{5}{*}{DeepFlow~\cite{weinzaepfel2013deepflow}} & YOLO11n & 01:01:37 & 0.7 & 2.6 & 6.3 & 0.118 & 0.050 & 0.154 & 0.058 \\
        & YOLO11s & 01:10:16 & 0.8 & 9.4 & 21.3 & 0.122 & 0.051 & 0.150 & 0.059 \\
        & YOLO11m & 01:43:47 & 1.1 & 20.0 & 67.6 & 0.123 & 0.052 & 0.156 & 0.061 \\
        & YOLO11l & 02:16:42 & 1.3 & 25.3 & 86.6 & 0.129 & 0.052 & 0.162 & 0.062 \\
        & YOLO11x & 02:54:47 & 1.6 & 56.8 & 194.4 & 0.132 & 0.055 & 0.163 & 0.063 \\
        \midrule
        \multirow{5}{*}{PCAFlow~\cite{wulff2015efficient}} & YOLO11n & 00:58:31 & 0.7 & 2.6 & 6.3 & 0.399 & 0.235 & 0.547 & 0.332 \\
        & YOLO11s & 01:08:27 & 0.8 & 9.4 & 21.3 & 0.413 & 0.252 & 0.547 & 0.332 \\
        & YOLO11m & 01:42:02 & 1.2 & 20.0 & 67.6 & 0.418 & 0.249 & 0.557 & 0.313 \\
        & YOLO11l & 02:17:19 & 1.3 & 25.3 & 86.6 & 0.416 & 0.253 & 0.525 & 0.326 \\
        & YOLO11x & 02:51:27 & 1.6 & 56.8 & 194.4 & 0.425 & 0.255 & 0.591 & 0.353 \\
        \midrule
        \multirow{5}{*}{DIS~\cite{kroeger2016fast}} & YOLO11n & 00:58:58 & 0.7 & 2.6 & 6.3 & 0.345 & 0.149 & 0.151 & 0.057 \\
        & YOLO11s & 01:08:51 & 0.8 & 9.4 & 21.3 & 0.336 & 0.149 & 0.149 & 0.056 \\
        & YOLO11m & 01:40:38 & 1.1 & 20.0 & 67.6 & 0.322 & 0.149 & 0.119 & 0.048 \\
        & YOLO11l & 02:16:17 & 1.3 & 25.3 & 86.6 & 0.358 & 0.158 & 0.153 & 0.060 \\
        & YOLO11x & 02:49:32 & 1.6 & 56.8 & 194.4 & 0.367 & 0.164 & 0.136 & 0.052 \\
        \midrule
        \multirow{5}{*}{\textbf{ReynoldsFlow (ours)}} & YOLO11n & 00:59:54 & 0.5 & 2.6 & 6.3 & 0.500 & 0.325 & 0.500 & 0.288 \\
        & YOLO11s & 01:08:42 & 0.6 & 9.4 & 21.3 & 0.493 & 0.282 & 0.666 & 0.370 \\
        & YOLO11m & 01:41:26 & 1.0 & 20.0 & 67.6 & 0.536 & 0.319 & 0.762 & 0.421 \\
        & YOLO11l & 02:15:58 & 1.3 & 25.3 & 86.6 & 0.528 & 0.304 & 0.722 & 0.335 \\
        & YOLO11x & 02:50:56 & 1.3 & 56.8 & 194.4 & 0.509 & 0.347 & 0.443 & 0.225 \\
        \bottomrule
    \end{tabular}
    % }
    \end{adjustbox}
    \caption{Comparison of YOLO11 performance on UAVDB across different optical flow methods with HSV space visualization.}
    \label{tab:experiments_uavdb_hsv}
\end{table*}

\begin{table*}
    % \small
    \centering
    % \resizebox{!}{\lineheight}{ % Adjust the table to the width of the page
    \begin{adjustbox}{max width=\textwidth, max height=0.5\textheight}
    \begin{tabular}{cccccccccc}
        \toprule
        \multirow{2}{*}{Methods} & \multirow{2}{*}{Model} & Training Time & Inference Time & \#Param. & FLOPs & \multirow{2}{*}{$\text{AP}^{val}_{50}$} & \multirow{2}{*}{$\text{AP}^{val}_{50-95}$} & \multirow{2}{*}{$\text{AP}^{test}_{50}$} & \multirow{2}{*}{$\text{AP}^{test}_{50-95}$}\\
            & & (hours:mins:sec) & (per image, ms) & (M) & (G) & \\
        \midrule
        \multirow{5}{*}{Horn-Schunck~\cite{horn1981determining}} & YOLO11n & 00:59:17 & 0.6 & 2.6 & 6.3 & 0.507 & 0.253 & 0.633 & 0.311 \\
        & YOLO11s & 01:08:39 & 0.7 & 9.4 & 21.3 & 0.472 & 0.236 & 0.652 & 0.313 \\
        & YOLO11m & 01:40:34 & 1.0 & 20.0 & 67.6 & 0.479 & 0.243 & 0.696 & 0.345 \\
        & YOLO11l & 02:14:24 & 1.3 & 25.3 & 86.6 & 0.451 & 0.220 & 0.613 & 0.295 \\
        & YOLO11x & 02:49:14 & 1.6 & 56.8 & 194.4 & 0.465 & 0.235 & 0.663 & 0.328 \\
        \midrule
        \multirow{5}{*}{Lucas-Kanade~\cite{lucas1981iterative}} & YOLO11n & 01:21:25 & 1.1 & 2.6 & 6.3 & 0.539 & 0.295 & 0.208 & 0.104 \\
        & YOLO11s & 01:23:11 & 1.2 & 9.4 & 21.3 & 0.580 & 0.323 & 0.236 & 0.115 \\
        & YOLO11m & 01:46:40 & 1.6 & 20.0 & 67.6 & 0.579 & 0.330 & 0.208 & 0.104 \\
        & YOLO11l & 02:19:01 & 1.8 & 25.3 & 86.6 & 0.594 & 0.324 & 0.220 & 0.108 \\
        & YOLO11x & 02:54:26 & 2.1 & 56.8 & 194.4 & 0.604 & 0.327 & 0.241 & 0.122 \\
        \midrule
        \multirow{5}{*}{Farneback~\cite{farneback2003two}} & YOLO11n & 00:58:33 & 0.7 & 2.6 & 6.3 & 0.840 & 0.547 & 0.682 & 0.444 \\
        & YOLO11s & 01:08:52 & 0.7 & 9.4 & 21.3 & 0.857 & 0.556 & 0.674 & 0.434 \\
        & YOLO11m & 01:40:49 & 1.1 & 20.0 & 67.6 & 0.841 & 0.548 & 0.693 & 0.446 \\
        & YOLO11l & 02:16:56 & 1.3 & 25.3 & 86.6 & 0.858 & 0.552 & 0.667 & 0.436 \\
        & YOLO11x & 02:48:47 & 1.6 & 56.8 & 194.4 & 0.843 & 0.546 & 0.719 & 0.481 \\
        \midrule
        \multirow{5}{*}{Brox~\cite{brox2004high}} & YOLO11n & 01:09:32 & 0.9 & 2.6 & 6.3 & 0.669 & 0.344 & 0.371 & 0.172 \\
        & YOLO11s & 01:12:16 & 1.0 & 9.4 & 21.3 & 0.672 & 0.350 & 0.362 & 0.173 \\
        & YOLO11m & 01:41:41 & 1.4 & 20.0 & 67.6 & 0.696 & 0.365 & 0.397 & 0.191 \\
        & YOLO11l & 02:16:09 & 1.5 & 25.3 & 86.6 & 0.698 & 0.363 & 0.413 & 0.197 \\
        & YOLO11x & 02:50:11 & 1.8 & 56.8 & 194.4 & 0.694 & 0.359 & 0.397 & 0.194 \\
        \midrule
        \multirow{5}{*}{TV-L1~\cite{zach2007duality}} & YOLO11n & 00:58:33 & 0.7 & 2.6 & 6.3 & 0.814 & 0.430 & 0.696 & 0.376 \\
        & YOLO11s & 01:07:53 & 0.7 & 9.4 & 21.3 & 0.814 & 0.435 & 0.705 & 0.403 \\
        & YOLO11m & 01:41:49 & 1.0 & 20.0 & 67.6 & 0.792 & 0.435 & 0.774 & 0.456 \\
        & YOLO11l & 02:14:29 & 1.3 & 25.3 & 86.6 & 0.820 & 0.451 & 0.748 & 0.431 \\
        & YOLO11x & 02:51:57 & 1.6 & 56.8 & 194.4 & 0.810 & 0.458 & 0.719 & 0.418 \\
        \midrule
        \multirow{5}{*}{SimpleFlow~\cite{tao2012simpleflow}} & YOLO11n & 00:54:13 & 0.7 & 2.6 & 6.3 & 0.491 & 0.265 & 0.460 & 0.234 \\
        & YOLO11s & 01:00:59 & 0.8 & 9.4 & 21.3 & 0.465 & 0.244 & 0.448 & 0.228 \\
        & YOLO11m & 01:31:20 & 1.0 & 20.0 & 67.6 & 0.444 & 0.242 & 0.367 & 0.197 \\
        & YOLO11l & 02:00:05 & 1.3 & 25.3 & 86.6 & 0.452 & 0.256 & 0.436 & 0.238 \\
        & YOLO11x & 02:32:22 & 1.6 & 56.8 & 194.4 & 0.460 & 0.262 & 0.400 & 0.205 \\
        \midrule
        \multirow{5}{*}{RLOF~\cite{senst2012robust}} & YOLO11n & 00:58:52 & 0.7 & 2.6 & 6.3 & 0.369 & 0.173 & 0.339 & 0.152 \\
        & YOLO11s & 01:06:55 & 0.8 & 9.4 & 21.3 & 0.360 & 0.170 & 0.337 & 0.146 \\
        & YOLO11m & 01:39:21 & 1.1 & 20.0 & 67.6 & 0.352 & 0.172 & 0.361 & 0.166 \\
        & YOLO11l & 02:14:01 & 1.3 & 25.3 & 86.6 & 0.354 & 0.170 & 0.375 & 0.172 \\
        & YOLO11x & 02:52:35 & 1.6 & 56.8 & 194.4 & 0.351 & 0.168 & 0.356 & 0.153 \\
        \midrule
        \multirow{5}{*}{DeepFlow~\cite{weinzaepfel2013deepflow}} & YOLO11n & 01:00:42 & 0.7 & 2.6 & 6.3 & 0.462 & 0.214 & 0.670 & 0.309 \\
        & YOLO11s & 01:09:31 & 0.8 & 9.4 & 21.3 & 0.478 & 0.221 & 0.663 & 0.309 \\
        & YOLO11m & 01:42:02 & 1.0 & 20.0 & 67.6 & 0.483 & 0.232 & 0.684 & 0.328 \\
        & YOLO11l & 02:16:08 & 1.3 & 25.3 & 86.6 & 0.441 & 0.201 & 0.702 & 0.340 \\
        & YOLO11x & 02:52:55 & 1.6 & 56.8 & 194.4 & 0.456 & 0.211 & 0.637 & 0.304 \\
        \midrule
        \multirow{5}{*}{PCAFlow~\cite{wulff2015efficient}}& YOLO11n & 00:58:47 & 0.7 & 2.6 & 6.3 & 0.492 & 0.247 & 0.657 & 0.328 \\
        & YOLO11s & 01:08:45 & 0.8 & 9.4 & 21.3 & 0.492 & 0.248 & 0.563 & 0.273 \\
        & YOLO11m & 01:42:26 & 1.1 & 20.0 & 67.6 & 0.498 & 0.241 & 0.674 & 0.342 \\
        & YOLO11l & 02:17:00 & 1.3 & 25.3 & 86.6 & 0.488 & 0.248 & 0.628 & 0.308 \\
        & YOLO11x & 02:50:41 & 1.6 & 56.8 & 194.4 & 0.457 & 0.229 & 0.665 & 0.328 \\
        \midrule
        \multirow{5}{*}{DIS~\cite{kroeger2016fast}} & YOLO11n & 01:01:05 & 0.9 & 2.6 & 6.3 & 0.435 & 0.199 & 0.555 & 0.260 \\
        & YOLO11s & 01:09:41 & 0.9 & 9.4 & 21.3 & 0.438 & 0.214 & 0.540 & 0.258 \\
        & YOLO11m & 01:42:19 & 1.1 & 20.0 & 67.6 & 0.444 & 0.215 & 0.597 & 0.286 \\
        & YOLO11l & 02:17:23 & 1.3 & 25.3 & 86.6 & 0.475 & 0.227 & 0.580 & 0.285 \\
        & YOLO11x & 02:51:21 & 1.6 & 56.8 & 194.4 & 0.479 & 0.234 & 0.611 & 0.304 \\
        \midrule
        \multirow{5}{*}{\textbf{ReynoldsFlow (ours)}} & YOLO11n & 00:58:31 & 0.6 & 2.6 & 6.3 & 0.910 & 0.571 & 0.895 & 0.547 \\
        & YOLO11s & 01:07:09 & 0.7 & 9.4 & 21.3 & 0.900 & 0.567 & \textbf{0.906} & 0.535 \\
        & YOLO11m & 01:39:57 & 1.1 & 20.0 & 67.6 & 0.909 & 0.572 & 0.893 & 0.573 \\
        & YOLO11l & 02:14:01 & 1.3 & 25.3 & 86.6 & 0.899 & 0.576 & 0.904 & \textbf{0.596} \\
        & YOLO11x & 02:51:50 & 1.6 & 56.8 & 194.4 & 0.902 & 0.569 & 0.831 & 0.507 \\
        \bottomrule
    \end{tabular}
    % }
    \end{adjustbox}
    \caption{Comparison of YOLO11 performance on UAVDB across different optical flow methods with enhanced flow visualization.}
    \label{tab:experiments_uavdb_enhanced}
\end{table*}

% \begin{table}
%     \centering
%     \begin{adjustbox}{max width=\linewidth}
%     \begin{tabular}{cccccc}
%         \toprule
%         \multirow{2}{*}{Methods} & \multirow{2}{*}{Split} & Training Time & \multirow{2}{*}{Average Loss} & \multirow{2}{*}{PCE}\\
%         & & (hours:mins:sec) & & \\
%         \midrule
%         \multirow{4}{*}{RGB} & 1 & 00:08:37 & 0.2354 & 0.708 \\
%         & 2 & 00:08:29 & 0.2275 & 0.688 \\
%         & 3 & 00:08:08 & 0.2289 & 0.715 \\
%         & 4 & 00:08:19 & 0.2334 & 0.708 \\
%         \midrule
%         \multirow{4}{*}{Grayscale} & 1 & 00:08:35 & 0.2496 & 0.711 \\
%         & 2 & 00:08:27 & 0.2435 & 0.679 \\
%         & 3 & 00:07:59 & 0.2432 & 0.699 \\
%         & 4 & 00:08:22 & 0.2542 & 0.703 \\
%         \bottomrule
%     \end{tabular}
%     \end{adjustbox}
%     \caption{Comparison of SwingNet performance on GolfDB with RGB and Grayscale inputs.}
%     \label{tab:experiments_golfdb_rgb_grayscale}
% \end{table}

\clearpage

\begin{table}
    % \small
    \centering
    \resizebox{\linewidth}{!}{ % Adjust table to the width of the page
    \begin{tabular}{cccccc}
        \toprule
        \multirow{2}{*}{Methods} & \multirow{2}{*}{Split} & Training Time & \multirow{2}{*}{Average Loss} & \multirow{2}{*}{PCE}\\
         & & (hours:mins:sec) & & \\
        \midrule
        \multirow{4}{*}{Horn-Schunck~\cite{horn1981determining}} & 1 & 00:08:09 & 0.2561 & 0.711 \\
        & 2 & 00:08:42 & 0.2545 & 0.704 \\
        & 3 & 00:08:23 & 0.2572 & 0.704 \\
        & 4 & 00:08:34 & 0.2548 & 0.709 \\
        \midrule
        \multirow{4}{*}{Lucas-Kanade~\cite{lucas1981iterative}} & 1 & 00:08:23 & 0.2315 & 0.690 \\
        & 2 & 00:08:04 & 0.2201 & 0.699 \\
        & 3 & 00:08:29 & 0.2316 & 0.687 \\
        & 4 & 00:08:35 & 0.2241 & 0.691 \\
        \midrule
        \multirow{4}{*}{Farneback~\cite{farneback2003two}} & 1 & 00:08:16 & 0.2559 & 0.705 \\
        & 2 & 00:08:33 & 0.2584 & 0.723 \\
        & 3 & 00:08:26 & 0.2483 & 0.718 \\
        & 4 & 00:08:35 & 0.2553 & 0.720 \\
        \midrule
        \multirow{4}{*}{Brox~\cite{brox2004high}} & 1 & 00:08:15 & 0.2484 & 0.708 \\
        & 2 & 00:08:38 & 0.2381 & 0.722 \\
        & 3 & 00:08:33 & 0.2401 & 0.699 \\
        & 4 & 00:08:33 & 0.2422 & 0.702 \\
        \midrule
        \multirow{4}{*}{TV-L1~\cite{zach2007duality}} & 1 & 00:08:44 & 0.1813 & \textbf{0.818} \\
        & 2 & 00:08:39 & 0.1785 & \textbf{0.811} \\
        & 3 & 00:08:33 & 0.1685 & \textbf{0.801} \\
        & 4 & 00:08:34 & 0.1791 & 0.811 \\
        \midrule
        \multirow{4}{*}{SimpleFlow~\cite{tao2012simpleflow}} & 1 & 00:08:32 & 0.2791 & 0.668 \\
        & 2 & 00:08:38 & 0.2764 & 0.658 \\
        & 3 & 00:08:34 & 0.2730 & 0.670 \\
        & 4 & 00:08:28 & 0.2814 & 0.664 \\
        \midrule
        \multirow{4}{*}{RLOF~\cite{senst2012robust}} & 1 & 00:08:50 & 0.2631 & 0.681 \\
        & 2 & 00:08:37 & 0.2463 & 0.655 \\
        & 3 & 00:08:36 & 0.2583 & 0.671 \\
        & 4 & 00:08:29 & 0.2570 & 0.663 \\
        \midrule
        \multirow{4}{*}{DeepFlow~\cite{weinzaepfel2013deepflow}} & 1 & 00:08:32 & 0.2154 & 0.725 \\
        & 2 & 00:08:37 & 0.2088 & 0.715 \\
        & 3 & 00:08:34 & 0.2119 & 0.698 \\
        & 4 & 00:08:28 & 0.2205 & 0.726 \\
        \midrule
        \multirow{4}{*}{PCAFlow~\cite{wulff2015efficient}} & 1 & 00:08:30 & 0.1919 & 0.772 \\
        & 2 & 00:08:39 & 0.1876 & 0.764 \\
        & 3 & 00:08:33 & 0.1858 & 0.758 \\
        & 4 & 00:08:30 & 0.1887 & 0.765 \\
        \midrule
        \multirow{4}{*}{DIS~\cite{kroeger2016fast}} & 1 & 00:08:36 & 0.1996 & 0.775 \\
        & 2 & 00:08:44 & 0.1936 & 0.786 \\
        & 3 & 00:08:35 & 0.2080 & 0.768 \\
        & 4 & 00:08:29 & 0.1969 & 0.760 \\
        \midrule
        \multirow{4}{*}{\textbf{ReynoldsFlow (ours)}} & 1 & 00:08:32 & 0.1734 & 0.806 \\
        & 2 & 00:08:38 & 0.1760 & 0.801 \\
        & 3 & 00:08:14 & 0.1793 & 0.795 \\
        & 4 & 00:08:28 & 0.1765 & \textbf{0.814} \\
        \bottomrule
    \end{tabular}
 }
    \caption{Comparison of SwingNet performance on GolfDB across different optical flow methods with HSV space visualization.}
    \label{tab:experiments_golfdb_hsv}
\end{table}

\begin{table}
    % \small
    \centering
    \resizebox{\linewidth}{!}{ % Adjust table to the width of the page
    \begin{tabular}{cccccc}
        \toprule
        \multirow{2}{*}{Methods} & \multirow{2}{*}{Split} & Training Time & \multirow{2}{*}{Average Loss} & \multirow{2}{*}{PCE}\\
         & & (hours:mins:sec) & & \\
        \midrule
        \multirow{4}{*}{Horn-Schunck~\cite{horn1981determining}} & 1 & 00:08:36 & 0.2012 & 0.762 \\
        & 2 & 00:08:19 & 0.1913 & 0.740\\
        & 3 & 00:08:02 & 0.1895 & 0.741\\
        & 4 & 00:08:20 & 0.2023 & 0.760\\
        \midrule
        \multirow{4}{*}{Lucas-Kanade~\cite{lucas1981iterative}} & 1 & 00:08:33 & 0.2179 & 0.759\\
        & 2 & 00:08:20 & 0.2010 & 0.729\\
        & 3 & 00:08:03 & 0.2012 & 0.737\\
        & 4 & 00:08:19 & 0.2085 & 0.743\\
        \midrule
        \multirow{4}{*}{Farneback~\cite{farneback2003two}} & 1 & 00:08:31 & 0.2169 & 0.755\\
        & 2 & 00:08:34 & 0.2122 & 0.751\\
        & 3 & 00:08:02 & 0.2116 & 0.762\\
        & 4 & 00:08:19 & 0.2100 & 0.750\\
        \midrule
        \multirow{4}{*}{Brox~\cite{brox2004high}} & 1 & 00:08:33 & 0.2351 & 0.727\\
        & 2 & 00:08:19 & 0.2228 & 0.717\\
        & 3 & 00:08:03 & 0.2197 & 0.710\\
        & 4 & 00:08:19 & 0.2257 & 0.725\\
        \midrule
        \multirow{4}{*}{TV-L1~\cite{zach2007duality}} & 1 & 00:08:44 & 0.1715 & 0.795\\
        & 2 & 00:08:36 & 0.1725 & 0.791\\
        & 3 & 00:08:04 & 0.1679 & 0.786\\
        & 4 & 00:08:27 & 0.1666 & 0.792\\
        \midrule
        \multirow{4}{*}{SimpleFlow~\cite{tao2012simpleflow}} & 1 & 00:08:33 & 0.2638 & 0.644\\
        & 2 & 00:08:20 & 0.2660 & 0.655\\
        & 3 & 00:08:03 & 0.2695 & 0.644\\
        & 4 & 00:08:10 & 0.2651 & 0.653\\
        \midrule
        \multirow{4}{*}{RLOF~\cite{senst2012robust}} & 1 & 00:08:42 & 0.2930 & 0.611\\
        & 2 & 00:08:36 & 0.2754 & 0.588\\
        & 3 & 00:08:05 & 0.2917 & 0.613\\
        & 4 & 00:08:23 & 0.2906 & 0.605\\
        \midrule
        \multirow{4}{*}{DeepFlow~\cite{weinzaepfel2013deepflow}} & 1 & 00:08:33 & 0.2445 & 0.693\\
        & 2 & 00:08:19 & 0.2239 & 0.671\\
        & 3 & 00:08:22 & 0.2380 & 0.667\\
        & 4 & 00:08:20 & 0.2305 & 0.667\\
        \midrule
        \multirow{4}{*}{PCAFlow~\cite{wulff2015efficient}} & 1 & 00:08:43 & 0.2169 & 0.713\\
        & 2 & 00:08:36 & 0.2136 & 0.718\\
        & 3 & 00:08:28 & 0.2136 & 0.709\\
        & 4 & 00:08:16 & 0.2150 & 0.702\\
        \midrule
        \multirow{4}{*}{DIS~\cite{kroeger2016fast}} & 1 & 00:08:33 & 0.2044 & 0.766\\
        & 2 & 00:08:19 & 0.1950 & 0.772\\
        & 3 & 00:08:14 & 0.1990 & 0.754\\
        & 4 & 00:08:21 & 0.2003 & 0.754\\
        \midrule % ReynoldsFlow_C
        \multirow{4}{*}{\textbf{ReynoldsFlow (ours)}} & 1 & 00:08:40 & 0.1851 & \textbf{0.808}\\
        & 2 & 00:08:28 & 0.1871 & \textbf{0.816}\\
        & 3 & 00:08:28 & 0.1883 & \textbf{0.816}\\
        & 4 & 00:08:28 & 0.1822 & \textbf{0.808}\\
        \bottomrule
    \end{tabular}
    }
    \caption{Comparison of SwingNet performance on GolfDB across different optical flow methods with enhanced flow visualization.}
    \label{tab:experiments_golfdb_enhanced}
\end{table}

% \begin{figure*}[tp]
%     \centering
%     \includegraphics[width=0.8\linewidth]{figs/appendix_fig1.jpg}
%     \caption{A detailed comparison of the two visualization approaches for each optical flow method is provided for two scenarios: frames 950 and 951 from Camera 0 in Dataset 1 and frames 1300 and 1301 from Camera 0 in Dataset 3.}
%     \label{fig:appendix_fig1}
% \end{figure*}
